# Supplementary material for: Anytime Continual Learning for Open Vocabulary Classification
Source: arXiv:2409.08518 source file (2024-09-13)
Supplement: Supplementary file 1 [file 6_suppl.tex]

\clearpage
%%%%%%%%%% Merge with supplemental materials %%%%%%%%%%
%%%%%%%%%% Prefix a "S" to all equations, figures, tables and reset the counter %%%%%%%%%%
\setcounter{section}{0}
\setcounter{equation}{0}
\setcounter{figure}{0}
\setcounter{table}{0}
\makeatletter

% \renewcommand{\bibnumfmt}[1]{[S#1]}
% \renewcommand{\citenumfont}[1]{S#1}
%%%%%%%%%% Prefix a "S" to all equations, figures, tables and reset the counter %%%%%%%%%%
\setcounter{page}{1}
% \maketitlesupplementary

% \section{More details}

% Most of our experiments are conducted on a single RTX 3090 GPU and an AMD Ryzen 9 5950X CPU. \zhen{Add more details here including the compression part.}

\section{Summary of contents}
The supplemental file contains more ablation experiments regarding sampling methods and the loss weight (Sec.~\ref{sec:sup_ablation}), details of different compression methods (Sec.~\ref{sec:compression_detail}), and a test under the MTIL task incremental learning setting established by ZSCL~\cite{ZSCL} for completeness (Sec.~\ref{sec:zscl_comparison}).

\section{Ablation experiments}
\label{sec:sup_ablation}

\begin{figure*}[!htb]
 \centering
 \begin{minipage}{\textwidth}
\includegraphics[width=\linewidth]{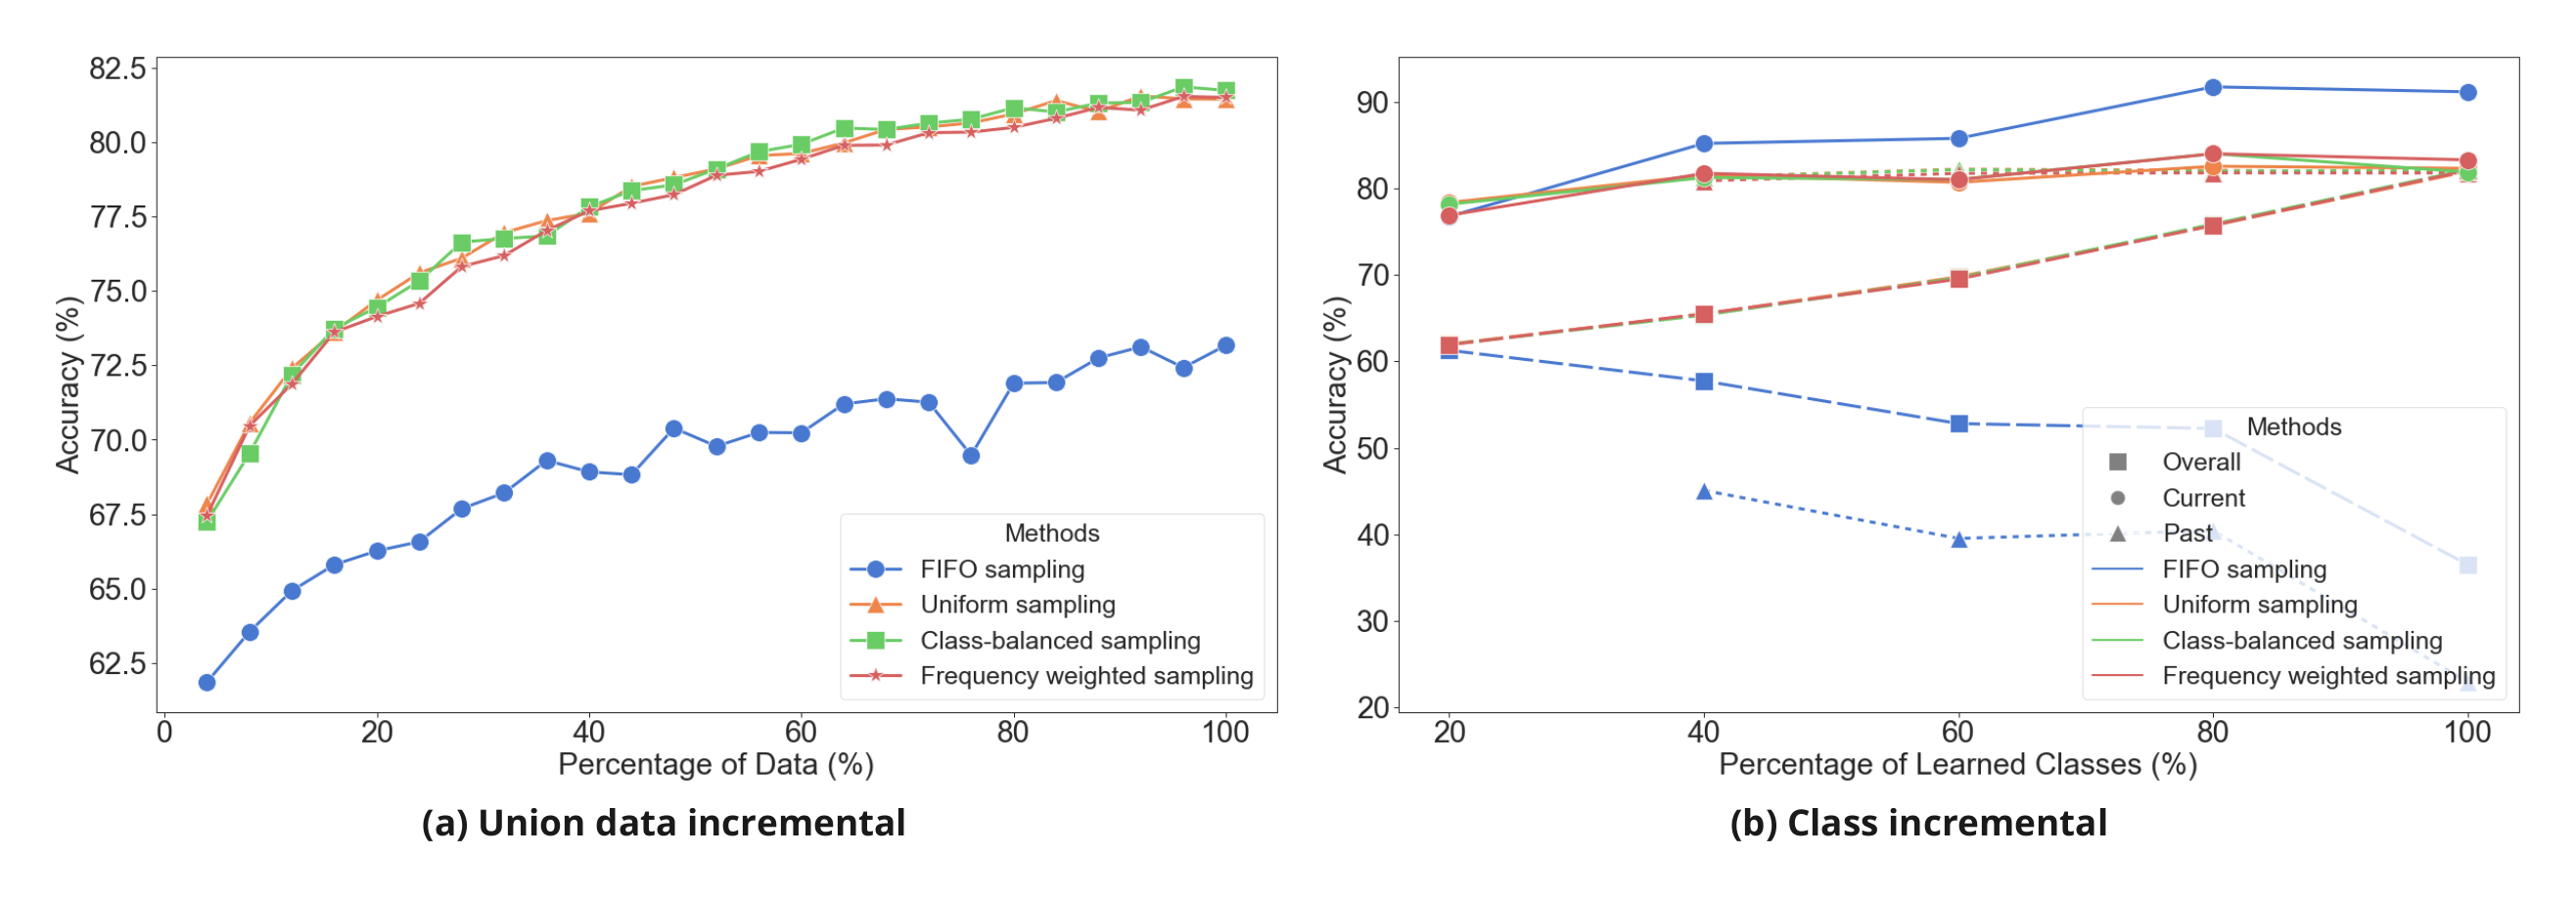}
\caption{Comparison of different sampling methods under the union data incremental (a) and class incremental learning (b) scenarios. All methods are trained online. Curves may overlay each other on (b) due to similar performances. Note that no ``past'' classes exist in the first stage of (b). In (b), we plot the accuracy for newly added classes (Current) and for classes seen before the stage began (Past). Note that overall classes include current, past and unseen classes. 
\label{fig:sampling}
}
\end{minipage}
\end{figure*}

\subsection{Ablation on different sampling methods}
As discussed in Sec.~3.3, our frequency weighted sampling works similarly as class balanced sampler and uniform random sampling. We also compare to first-in-first-out (FIFO) sampling, which only provides recent samples to the model. The comparison is useful to identify whether having access to all data is more effective for anytime continual learning. 

In our online training setup, each training data batch includes one new sample, with the rest of the batch composed according to different sampling strategies. We initially evaluated these methods in the data incremental learning context of a union of target tasks (union data incremental), as shown in Fig.~\ref{fig:sampling} (a). FWS, class-balanced, and uniform sampling demonstrated similar performance across all timestamps, consistently outperforming FIFO sampling. This outcome highlights the importance of retaining access to the entire exemplar set for continual improvement.

Moreover, FWS distinguishes itself by assigning higher probabilities to more recent samples, potentially benefiting scenarios requiring rapid adaptation to new data while maintaining reasonable performance on older tasks. We regard class incremental learning an apt test case for this. As shown in Fig.~\ref{fig:sampling} (b), besides the overall stage accuracy, we also plot the accuracy for newly added classes (Current) and for classes seen before the stage began (Past). From the plot, FIFO sampling has the highest current accuracy but falls short in past accuracy. FWS has a relatively higher current accuracy in later stages along with robust past accuracy, compared to Uniform and Class-balanced sampling. While we do not assert that FWS uniquely outperforms other sampling methods in every aspect, its adjustable weighting mechanism offers versatility for various applications.

\subsection{Ablation on decay multiplier $\xi$ of FWS}

\begin{table}
\centering
\caption{Performance of different $\xi$ in union data incremental learning and class incremental learning scenarios. All experiments adopt the online training setting. Result in the table is the average accuracy across all target tasks after receiving all data.}
\begin{tabular}{lcc}
\toprule
{Decay multiplier $\xi$} & {Data-Inc. Acc.} & {Class-Inc. Acc.}\\
\midrule
1.00 & 81.5 & 82.0 \\
0.99 & 81.5 & 82.1 \\
0.95 & 81.8 & 81.3 \\
0.90 & 81.7 & 80.2 \\
0.85 & 81.4 & 80.5 \\
0.80 & 81.6 & 81.0 \\
0.75 & 81.6 & 81.0 \\
0.70 & 81.6 & 81.7 \\
\bottomrule
\end{tabular}
\label{tab:decay_multiplier}
\end{table}

% \vspace{2mm} \noindent \textbf{Ablation on decay multiplier $\xi$.}~
Another hyperparameter influential to our frequency weighted sampling method is the decay multiplier $\xi$, which adjusts the sampling weight on recent data. We evaluate different $\xi$ values in the union data incremental and class incremental learning scenarios. Results are depicted in Tab.~\ref{tab:decay_multiplier}. We find different $\xi$ leads to minor differences for the union data incremental learning setting but the difference on class incremental learning setting is more obvious. $\xi=0.99$ demonstrates robust performance in class incremental learning. Therefore, we have set $\xi=0.99$ as the default value in our method.

% We illustrate the comparison in Fig.~\ref{fig:sampling}.

% \section{Ablation experiments}
% To perform the following experiments, we create a union of data from all tasks and then perform online learning with the corresponding configurations. The results are reported as the average accuracy across all target tasks.

% \subsubsection{Ablation on loss weight $\beta$}

\subsection{Abltion on loss weight $\beta$}
\begin{table}
\centering
\caption{Performance of various $\beta$ using online learning and offline learning. For online accuracy, the result is the average of accuracy on all target tasks after all data is received (union data incremental). For offline accuracy, the result is obtained by training the model for 32 epochs on the union of all target tasks.}
\begin{tabular}{lcc}
\toprule
Loss weight $\beta$ & {Online Acc.}  & Offline Acc. \\
\midrule
0.0 & 80.9 & 82.2 \\
0.1 & 81.5 & 83.0 \\
0.2 & 81.5 & 82.9 \\
0.3 & 81.5 & 82.9 \\
0.4 & 81.6 & 82.9 \\
0.5 & 81.6 & 82.9 \\
0.6 & 81.6 & 82.8 \\
0.7 & 81.6 & 82.6 \\
0.8 & 81.5 & 82.3 \\
0.9 & 81.6 & 82.2 \\
1.0 & 81.5 & 82.2 \\
% \rowcolor{yellow} 0.1 & \textbf{82.517} \\
\bottomrule
\end{tabular}
\label{tab:loss_weight}
\end{table}

% \vspace{2mm} \noindent \textbf{Ablation on loss weight $\beta$.}~
In Sec.~3.4, we introduce a loss term to prioritize the ``other'' logit over other incorrect labels, facilitating efficient out-of-domain sample confidence estimation. Our experimental results verify that the ``other'' logit alone works as an effective weighting method. Here, we show that even without explicitly using the ``other'' logit for weighting, this loss term independently enhances overall performance. 

In our experimental setup, we keep consistent configurations while varying the loss weight $\beta$ to assess its impact. 
We combine training data from all target tasks for both single-stage online and offline learning. For offline learning, we train the model for 32 epochs to keep the same number of training iterations as online learning. For the simplicity of result analysis, we choose PCW as the weighting method due to its independence from $p_{\text{other}}$. The results, depicted in Tab.~\ref{tab:loss_weight}, reveal a notable decline in performance when the loss weight is set to 0, indicating the absence of the loss term during training. Performance remains relatively stable for $0 < \beta < 0.7$. However, a decrease in offline accuracy is observed for $\beta > 0.7$. Consequently, we chose $\beta=0.1$ as the default setting, given its balanced accuracy in both online and offline scenarios.

% Though DCW has similar performance with PCW described in Sec. 4.3 from our evaluation in our main paper, the loss (weighted by $\beta$) used to encourage higher score for the ``other'' logit is useful for the performance for either online and offline learning. 
% To test the impact of different $\beta$s,

% It should be noted that when $\xi=1$, frequency weighted sampling is equivalent to uniform sampling. Another extreme is when $\xi$ is small enough, \eg, $\xi=w_{\text{min}}$, FWS is also equivalent to uniform sampling. It is noticeable that most $\xi$ lead to better performance than uniform sampling. 
% $\xi=0.99$ shows a reasonable performance particularly in class incremental learning. Consequently, we adopt $\xi=0.99$ as the default setting.

\section{Compression method detail}
\label{sec:compression_detail}

In this section, we complement more details of methods and implementation of Tab.~1 in the main paper.

\vspace{2mm} 
\noindent \textbf{Full Image.}~CLIP reshapes the input image to resolution $224\times 224$ and then creates $32\times32$ non-overlapping patches, resulting $7\times 7$ feature vectors (tokens) to the transformer network. Along with the CLS token attached to the start of the token sequence, the shape of the transformer network output is $50 \times D$, where $D$(=768 in our case) represents the feature vector dimension. For classification, we only leverage the CLS token. For fair comparison with other methods in the results of Tab.~1, we partially fine-tune the last layer of the transformer block. Processing a batch includes image loading, processing, a complete forward pass, and a backward pass restricted to the final layer.

\vspace{2mm} 
\noindent \textbf{Full Features.}~We pre-compute the intermediate features ($50 \times D$) before the final layer on all data and then store them to disk. For fine-tuning, we load stored features back from disk to RAM and feed them directly into the final layer, which is the only layer tuned. Processing a batch includes loading intermediate features, forward and backward pass of the final layer.

\vspace{2mm} 
\noindent \textbf{VQ.}~For Vector Quantization, we pre-train a codebook on intermediate features before the final layer using MSE loss between the quantized features and the original features. We adopt Zheng~\etal.~\cite{cvq-vae_iccv_2023}'s method to enhance VQ performance by promoting the use of more codebook vectors. Then, we process all images in the dataset to obtain the corresponding codebook indices. We store the codebook and indices of all samples to disk. Similar to Full Features, when fine-tuning, data processing involves loading a codebook and integer indices of intermediate features into RAM for feature reconstruction. To process a single batch, we need codebook and indices loading, feature reconstruction by retrieving codewords from the codebook according to the indices, forward and backward pass of the final layer.

\vspace{2mm} \noindent \textbf{PCA.}~Assume $f$ is the data to compress. We first center $f$ by subtracting the mean values of each token: $\hat{f} = f - \mu$, where $\mu$ represent the mean values of all tokens. We follow scikit-learn to perform SVD on $\hat{f}$: $\hat{f} = \mathbf{U} \mathbf{\Sigma} \mathbf{V}^T$. The reduced form of $\hat{f}$ can be approximated by $\hat{f}\approx \mathbf{U}_n \mathbf{\Sigma}_n \mathbf{V}_n^T$, where $n$ is the number of principal components/singular values chosen. $\mathbf{U}_n \mathbf{\Sigma}_n $ is the PCA coefficient matrix and $\mathbf{V}_n^T$ is the PCA component matrix. Ideally, we want to find a small $n$ so that the accuracy after fine-tuning is reasonably good. To reconstruct the data, we perform: $\mathbf{U}_n \mathbf{\Sigma}_n \mathbf{V}_n^T + \mu$.

\vspace{2mm} 
\noindent \textbf{Dataset-wide PCA.}~Since the intermediate feature is of shape $50\times D$ and in our case $D=768>50$, it makes a higher compression rate to compress along the vector dimension. For dataset-wide PCA, we concatenate the intermediate features from all samples together along the dimension of the 50 tokens and then apply PCA on the whole concatenated feature. Due to hardware limitation of RAM capacity, processing the whole dataset is not feasible. Therefore, we divide the whole dataset into chunks of 5,000 samples each. PCA is performed on each chunk and we store feature means, PCA coefficients, and components to disk. Processing a single batch involves loading these data from disk to RAM, reconstructing features via PCA, and processing them through the final layer (both forward and backward pass).

\vspace{2mm} 
\noindent \textbf{Per-instance PCA.}~For this method, PCA is applied on the 50 tokens of {\em each sample}. We store the feature means, PCA coefficients, and components to disk. The procedures required to process a batch are similar as dataset-wide PCA.

\vspace{2mm} 
\noindent \textbf{CLS-weight.}~As introduced earlier in this section, the CLS token is used for classification after the final layer. Our intuition is in the compression process, tokens similar to the CLS token are more crucial for classification performance. Our CLS-weight method involves reweighting the other tokens based on their similarity to the CLS token. This similarity is assessed using the first row of the affinity matrix (dimensions $50 \times 50$) from the self-attention module in the final layer. We then multiply the tokens with the corresponding similarities. Following this reweighting, per-instance PCA is applied to the adjusted intermediate feature.

\vspace{2mm} 
\noindent \textbf{Int-quantization.}~To reduce memory usage, we convert principal components from 32-bit floats to 8-bit integers, potentially reducing memory by approximately fourfold. We perform min-max normalization for each vector and map it to uint8 (0–255). We store the min-max values alongside the uint8 vector. Reconstruction involves mapping the vector back to float numbers. A similar process can be applied to principal coefficients, although the memory savings are less significant.

\vspace{2mm} \noindent \textbf{Implementation details.}~We run the same test 100 times for each method without other ongoing programs, and then compute the mean as the result of the time needed to process a single batch. We perform partial fine-tuning on the final block of the transformer network. We opt for a batch size of 32, a learning rate of 5e-6, a weight decay of 0.05, and conduct fine-tuning over 10 epochs.

\input{tables/diff_components}

\vspace{2mm} \noindent \textbf{Impact of number of components used for per-instance PCA.}~As default, we use only 5 components for per-instance PCA in Tab.~1. Here, we additionally present results using 3, 10, and 20 components in Tab.~\ref{tab:different_components}. For 3 components, compression is around 2/3 of 5 components but its FT accuracy for all three methods drops. The gains of introducing more components than 5 are not significant. Therefore, we use 5 components as default.

\begin{table}
\centering
\scalebox{1}{
\begin{tabular}{lcc}
\toprule
No. components &  FT Accuracy & KB/example\\
\midrule
100 & 74.9 & 20.1\\
200 & 76.3 & 40.2\\
300 & 77.1 & 60.1\\
400 & 77.4 &  80.2\\
500 & 77.6 &  100.3\\
\bottomrule
\end{tabular}
}
\caption{Dataset-wide fine-tuning accuracy with different components. 
% \zhen{Also, can we include KB/example here?}
\label{tab:dataset_different_components}}
\end{table}

\vspace{2mm} \noindent \textbf{Impact of number of components used for Dataset-wide PCA.}~In the paper, we use 200 components for compression since it gives a decent compression rate. Ideally, using more components gives better performance with a compromise on the compression rate, as shown in Tab.~\ref{tab:dataset_different_components}. 

\section{Test under MTIL task incremental learning~\cite{ZSCL}}
\label{sec:zscl_comparison}

\input{tables/detailed_results_under_zscl}

We also present the detailed accuracies of our method in Tab.~\ref{tab:anytimeCL_online_zscl} and Tab.~\ref{tab:anytimeCL_wake_sleep_zscl}. Our internal tests revealed that hyperparameter tuning, such as adjusting the learning rate for each task, can enhance results, as revealed in {\href{https://github.com/Thunderbeee/ZSCL/tree/8cd0caf19dfbb024dcde3fb3af8adbf6949259e8}{ZSCL's released code}}~\cite{ZSCL}. However, we tend to avoid hyperparameter tuning of different tasks since selected hyperparameters do not guarantee a better performance when the data distribution in an online data stream shifts.
